# Supplementary material for: Ultrafast non-thermal laser excitation of gigahertz longitudinal and shear acoustic waves in spin-crossover molecular crystals [$Fe(PM-AzA)_{2}$$(NCS)_{2}$]
Source: arXiv:1604.03297 source file (2017-10-17)
Supplement: Supplementary file 1 [file Supp_Final_reply.pdf]

# Supplementary Material for “Ultrafast non-thermal laser excitation of gigahertz longitudinal and shear acoustic waves in spin-crossover molecular crystals $[Fe(PM - AzA)_2(NCS)_2]$ ”

## I. WHITE LIGHT ELLIPSOMETRY

In order to access the optical properties of  $Fe(PM - AzA)_2(NCS)_2$  molecular crystals, we have conducted white light ellipsometry measurements across the spin-crossover temperature. The refractive indexes at 400 nm pump and 800 nm probe wavelengths extracted from the ellipsometry measurements are displayed in Fig. S1. The real  $n$  and imaginary  $k$  parts of the optical index were extracted from measurements of the  $4 \times 4$  Mueller matrices using the Berreman formalism [1] as described by [2]. The conventions  $\parallel$  and  $\perp$  used as a subscript for the indices notations in Fig. S1, refer to the probe polarization either parallel  $\parallel$  or perpendicular  $\perp$  to the optical plane of incidence which contains the crystal axis  $c$ .

The general tendency of a slight decrease of the real part  $n$  of the index of refraction at increasing temperatures is consistent with the fact that the material is less dense at higher temperature. Concerning the imaginary part  $k$  of the material, we can notice a strong discrepancy between 400 nm and 800 nm wavelengths which emphasizes that the crystal is significantly more absorbing at the pump wavelength than at the probe wavelength. As a general rule, these data evidence that the refractive index does not change significantly with temperature. We can notice as well a difference in the index of refraction for parallel  $\parallel$  or perpendicular  $\perp$  light polarizations that is linked to the optical anisotropy of the compound.

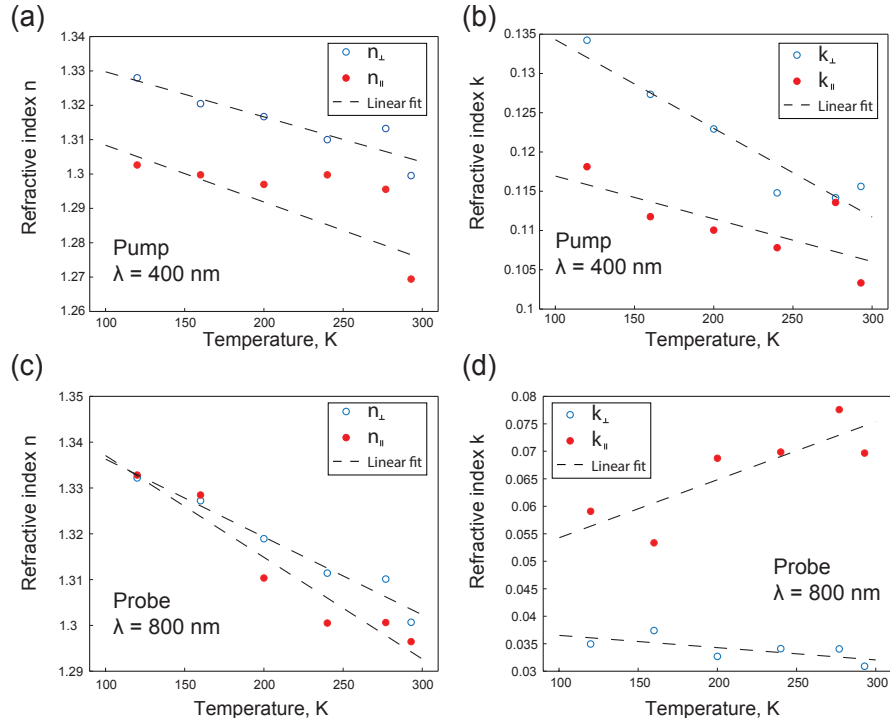

Fig. S1: (a) Real  $n$  and (b) imaginary  $k$  parts of the refractive index at 400 nm pump wavelength. (c) Real  $n$  and (d) imaginary  $k$  parts of the refractive index at 800 nm probe wavelength. The data were obtained at different crystal temperatures across the spin-crossover temperature and for two different polarizations parallel  $\parallel$  or perpendicular  $\perp$  to the optical plane of incidence.

## II. TRANSIENT REFLECTIVITY VERSUS DEPOLARIZED BRILLOUIN SCATTERING

Time domain Brillouin scattering enables the optical detection of coherent acoustic phonons in transparent or semi-transparent materials. Upon scattering of the probe light from propagating acoustic phonons, the detected signal highlights time domain oscillations at the Brillouin frequency of the scattering material. As in any Brillouin scattering process, the frequency  $\nu$  of these oscillations is related to the ultrasound velocity  $v$  of the material, to the probe wavelength  $\lambda$ , to the refractive index  $n$  of the medium, and to the back-scattering angle  $\theta$  through

$$\nu = 2 n v \cos \theta / \lambda. \quad (\text{S1})$$

Since the ultrasonic speeds  $v$  of longitudinal and shear acoustic phonons are different, the corresponding Brillouin frequencies can be separated in the detected signals. In fact, the detection rules for shear acoustic phonons are not as straightforward than for longitudinal acoustic phonons [3]. The detection of longitudinal acoustic waves can be performed through interferometric, deflectometric or reflectometric techniques. The reflectometric detection technique is sensitive to any phenomenon that modifies the optical properties of the material such as the pressure or change in density following the longitudinal acoustic phonons. Since shear acoustic waves do not modify the density in isotropic materials, the reflectometric detection technique which measures the change in probe intensity of the probe light is in general not sensitive to shear acoustic phonons. The alternative is to detect the flip of probe polarization, which is caused by shear phonons only, rather than reflectometry. This detection technique is sometimes referred to by the name depolarized Brillouin scattering, ellipsometric or MOKE detection (the optical scheme for the shear detection is identical to the Magneto-Optic Kerr angle measurement in magnetometry). In the present molecular crystal, which is highly anisotropic, the well-established rules for the detection of shear acoustic phonons in isotropic materials are still relevant. Fig. S2 compares experimentally both detection techniques, reflectometry and depolarized Brillouin scattering. As noticed in the frequency spectrums displayed in Fig. S2(b) and S2(c), the detected shear amplitude is enhanced in case of depolarized Brillouin scattering, which agrees well with the above mentioned general rules for shear acoustic detection. To conclude, the fact that the sensitivity of the shear acoustic detection varies between reflectometry and depolarized Brillouin scattering is a confirmation of the acoustic nature of the detected frequencies in our signals.

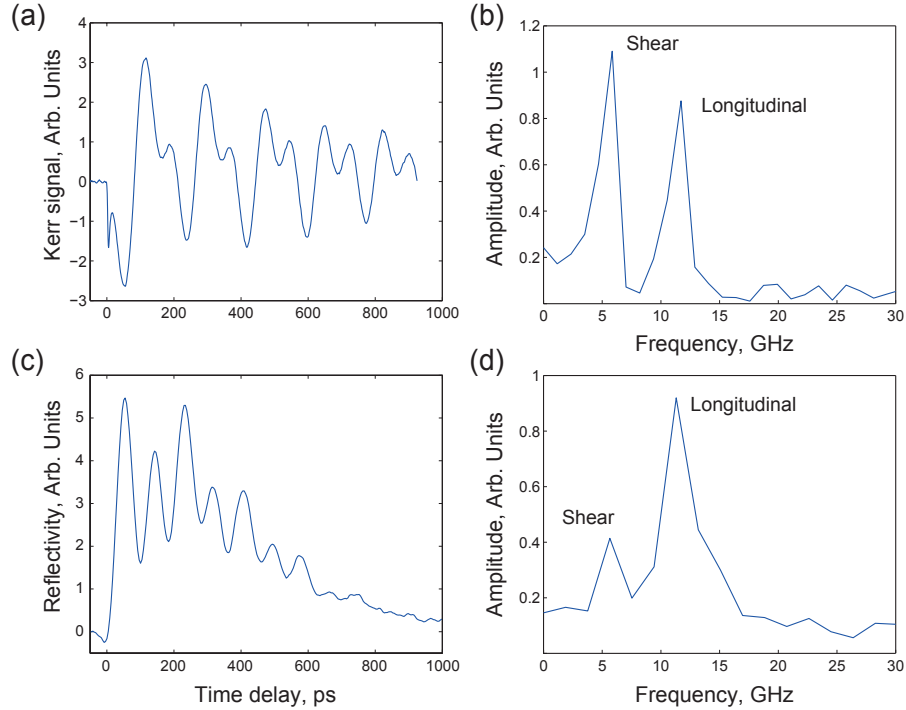

Fig. S 2: Transient depolarized Brillouin scattering signal (a) and its corresponding frequency spectrum (b) recorded in the molecular crystal. Transient reflectivity signal (c) and its corresponding frequency spectrum (d). The data were measured at oblique probe incidence with a 400 nm pump and a 800 nm probe, at room temperature.

- 
- [1] D. W. Berreman, J. Opt. Soc. Am. **62**, 502 (1972).
  - [2] G. Jellison, M. McGuire, L. Boatner, J. Budai, E. Specht, D. Singh, Phys. Rev. B **84**, 195439 (2011).
  - [3] T. Pezeril, J. Opt. Laser Technol. **83**, 177 (2016).
